# Supplementary material for: On Finding Gray Pixels
Source: arXiv:1901.03198 source file (2019-05-02)
Supplement: Supplementary file 1 [file supplement.tex]

\section{Detailed settings of learning-based methods}
\label{sec:detailed_setting}

To evaluate the performance of learning-based method in camera-agnostic scenario, we re-run the Bayesian method \cite{gehler2008bayesian}, Chakrabarti \textit{et al.} 2015~\cite{chakrabarti2015color}, FFCC \cite{barron2017fourier}, and the method by Cheng \textit{et al.} 2015 \cite{cheng2015effective}, using the codes provided by the authors. FFCC shows the best overall performance in the camera-known setting. Our experimental settings for re-running the aforementioned algorithms are summarized below:

\begin{tabular}{p{0.4\linewidth}p{0.5\linewidth}}
\textbf{Bayesian method \cite{gehler2008bayesian}} & Among all variations of Bayesian methods stated in \cite{gehler2008bayesian}, we use Bayes (GT) but without indoor/outdoor split, to which Bayes (tanh) is sensible. The ground truth of training illuminations (\textit{e.g.} Gehler-Shi) is used as point-set prior for testing on the other dataset (\textit{e.g.} NUS 8-camera)\\
\textbf{Chakrabarti \etal 2015~\cite{chakrabarti2015color}} & We use both variations given by the author: the empirical and the end-to-end trained method. We keeps all training hyperparameters same, \textit{e.g.} epoch number, momentum and learning-rate for SGD.\\
\textbf{FFCC \cite{barron2017fourier}} & For fair comparison, we use Model (J) (FFCC full,4 channels) in \cite{barron2017fourier}, which is free of camera metadata and semantic information but still state-of-the-art.\\
\textbf{Cheng \etal 2015 \cite{cheng2015effective}} & Same as \cite{cheng2015effective}, we use four 2D features with an ensemble of regression trees (K=30).
\end{tabular}

\section{Uniform black level and saturation correction}
\label{sec:unifromblacklevel}
Since the original learning-based methods mentioned previously in Section \ref{sec:detailed_setting} do not share the same process to correct black-level offset and pixel saturation, we implemented a unique pre-processing pipeline for all the methods. Although this implementation detail is often neglected in the literature, we realized that this can change slightly the linear relationship between the scene illumination and the captured image values. Table \ref{tab:black_satu} summarizes black level $B$ and saturation level $S$ for each camera of the Gehler-Shi and NUS 8-camera datasets. In this work, we pre-process all images as:

\begin{equation}
I_i^{(x,y)} = \max\left\lbrace 0, I_i^{(x,y)}-\textit{B} \right\rbrace, 
\label{eq:bl_correction}
\end{equation}
\begin{equation}
I_i^{(x,y)} = \min\left\lbrace 1, \frac{I_i^{(x,y)} }{0.95\textit{S}-\textit{B}} \right\rbrace,
\label{eq:bl_correction}
\end{equation}
 
 In addition, we include a boolean mask $M^{(x,y)}$ aimed at discarding very dark pixels for subsequent analysis:

\begin{equation}
M^{(x,y)} =
\begin{cases}
    1,& \vert I \vert^{(x,y)} \leq 0.0315 \times \max(I) \\
    0,& \text{otherwise}
\end{cases}
\label{eq:mask_bl_sl}
\end{equation}

\begin{table*}
\vspace{-0.4cm}
\caption{Black level and Saturation level for each camera of two benchmarks.} 
\label{tab:black_satu}
\begin{center}
\scriptsize
  \begin{tabular}{l rr || rrrrrrrr}
    \toprule 
  &  \multicolumn{2}{c}{Gehler-Shi} & \multicolumn{8}{c}{NUS 8-camera}\\
 & Canon & Canon  & Canon & Canon & Fujifilm & Nikon& Olympus & Panasonic & Samsung & Sony \\
 &  1D & 5D  & 1DS Mark3 & 600D & X-M1 & D5200 & E-PL6 & DMC-GX1 & NX2000 & SLT-A57 \\
 \midrule
 
\textit{B} & 0 & 129 & 1024 & 2048  & 256 & 0 & 255 & 143 & 0 & 128 \\
\textit{S} & 4095 & 4095 & 15279 & 15303  & 4079 & 15892 & 4043 & 4095 & 4095 & 4093 \\
% GP$^\ast$ & 4.1 &  2.5 & 2.8  & 5.1 & 2.2 & 2.7  \\ 
\bottomrule
  \end{tabular}
\end{center}\vspace{-0.8cm}
\end{table*}
 
 \section{More Visual Results}
 \begin{itemize}
    \item See Fig. \ref{figure:mimo_supple} for More visual results on spatial-illumination MIMO benchmark.
    \item See Fig. \ref{fig:single_illu_supple} for More visual results on single-illumination Gehler-Shi benchmark.
     \item See Fig. \ref{fig:single_illu_nus_supple} for More visual results on single-illumination NUS 8-camera benchmark. 
\end{itemize}

\input{fig_mimo_supple.tex}
\input{fig_single_supple.tex}
\input{fig_single_nus_supple.tex}
